# Supplementary material for: Redesigning Out-of-Distribution Detection on 3D Medical Images
Source: arXiv:2308.07324 source file (2023-08-07)
Supplement: Supplementary file 1 [file 9_appendix.tex]

\textbf{Adaptation of methods and implementation details}

Here, we detail the implementation of selected methods. \textbf{Baseline} is calculated using both maximum and entropy of the model output (U-Net with softmax) per image. \textbf{Deep Ensembles} are represented by $3$ U-Net models. \reconsider{Our experiments show that $3$ models is enough.} We calculate voxel-wise standard deviations to measure disagreement of predictions as such aggregation performed better than BALD \citep{houlsby2011bayesian} in our experiments. \textbf{MC-dropout} is implemented by introducing a dropout layer before every downsampling and upsampling operations in the U-Net model. We calculate voxel-wise standard deviations for $10$ inference steps with dropout rate of $0.1$. For all these methods we average voxel-wise scores for the whole image to obtain a single OOD score. \textbf{SVD} method is implemented without changes.

\reconsider{GODIN method was initially designed for classification \citep{hsu2020generalized}, thus, we detail its adaptation to segmentation. The dividend/divisor structure of the output layer that produces logit map $F_i(x)$ for class $i$ and image $x$ is kept the same:

\begin{equation}
    F_i(x) = \frac{H_i(x)}{G(x)}.
\end{equation}

Logits $F(x)$ are then normalized by the exponential
function (i.e. softmax) for outputting a class probability. $H_i(x)$ is taken from the initial U-Net architecture without changes: it is $H(x) = BN(ReLU(Conv(x, C)))$: convolutional layer with $C$ ($C$ is number of classes) output channels is followed by an activation and batch normalization. Similarly to the original paper, $G(x) = \sigma \left(BN(ReLU(Conv(x, 1)))\right)$. As a result, $G(x)$ is an uncertatinty map, which is then averaged to get a single image-wise score for out-of-distribution detection.}
